# Supplementary material for: Privacy-Preserving Video Conferencing via Thermal-Generative Images
Source: arXiv:2303.09279 source file (2023-03-28)

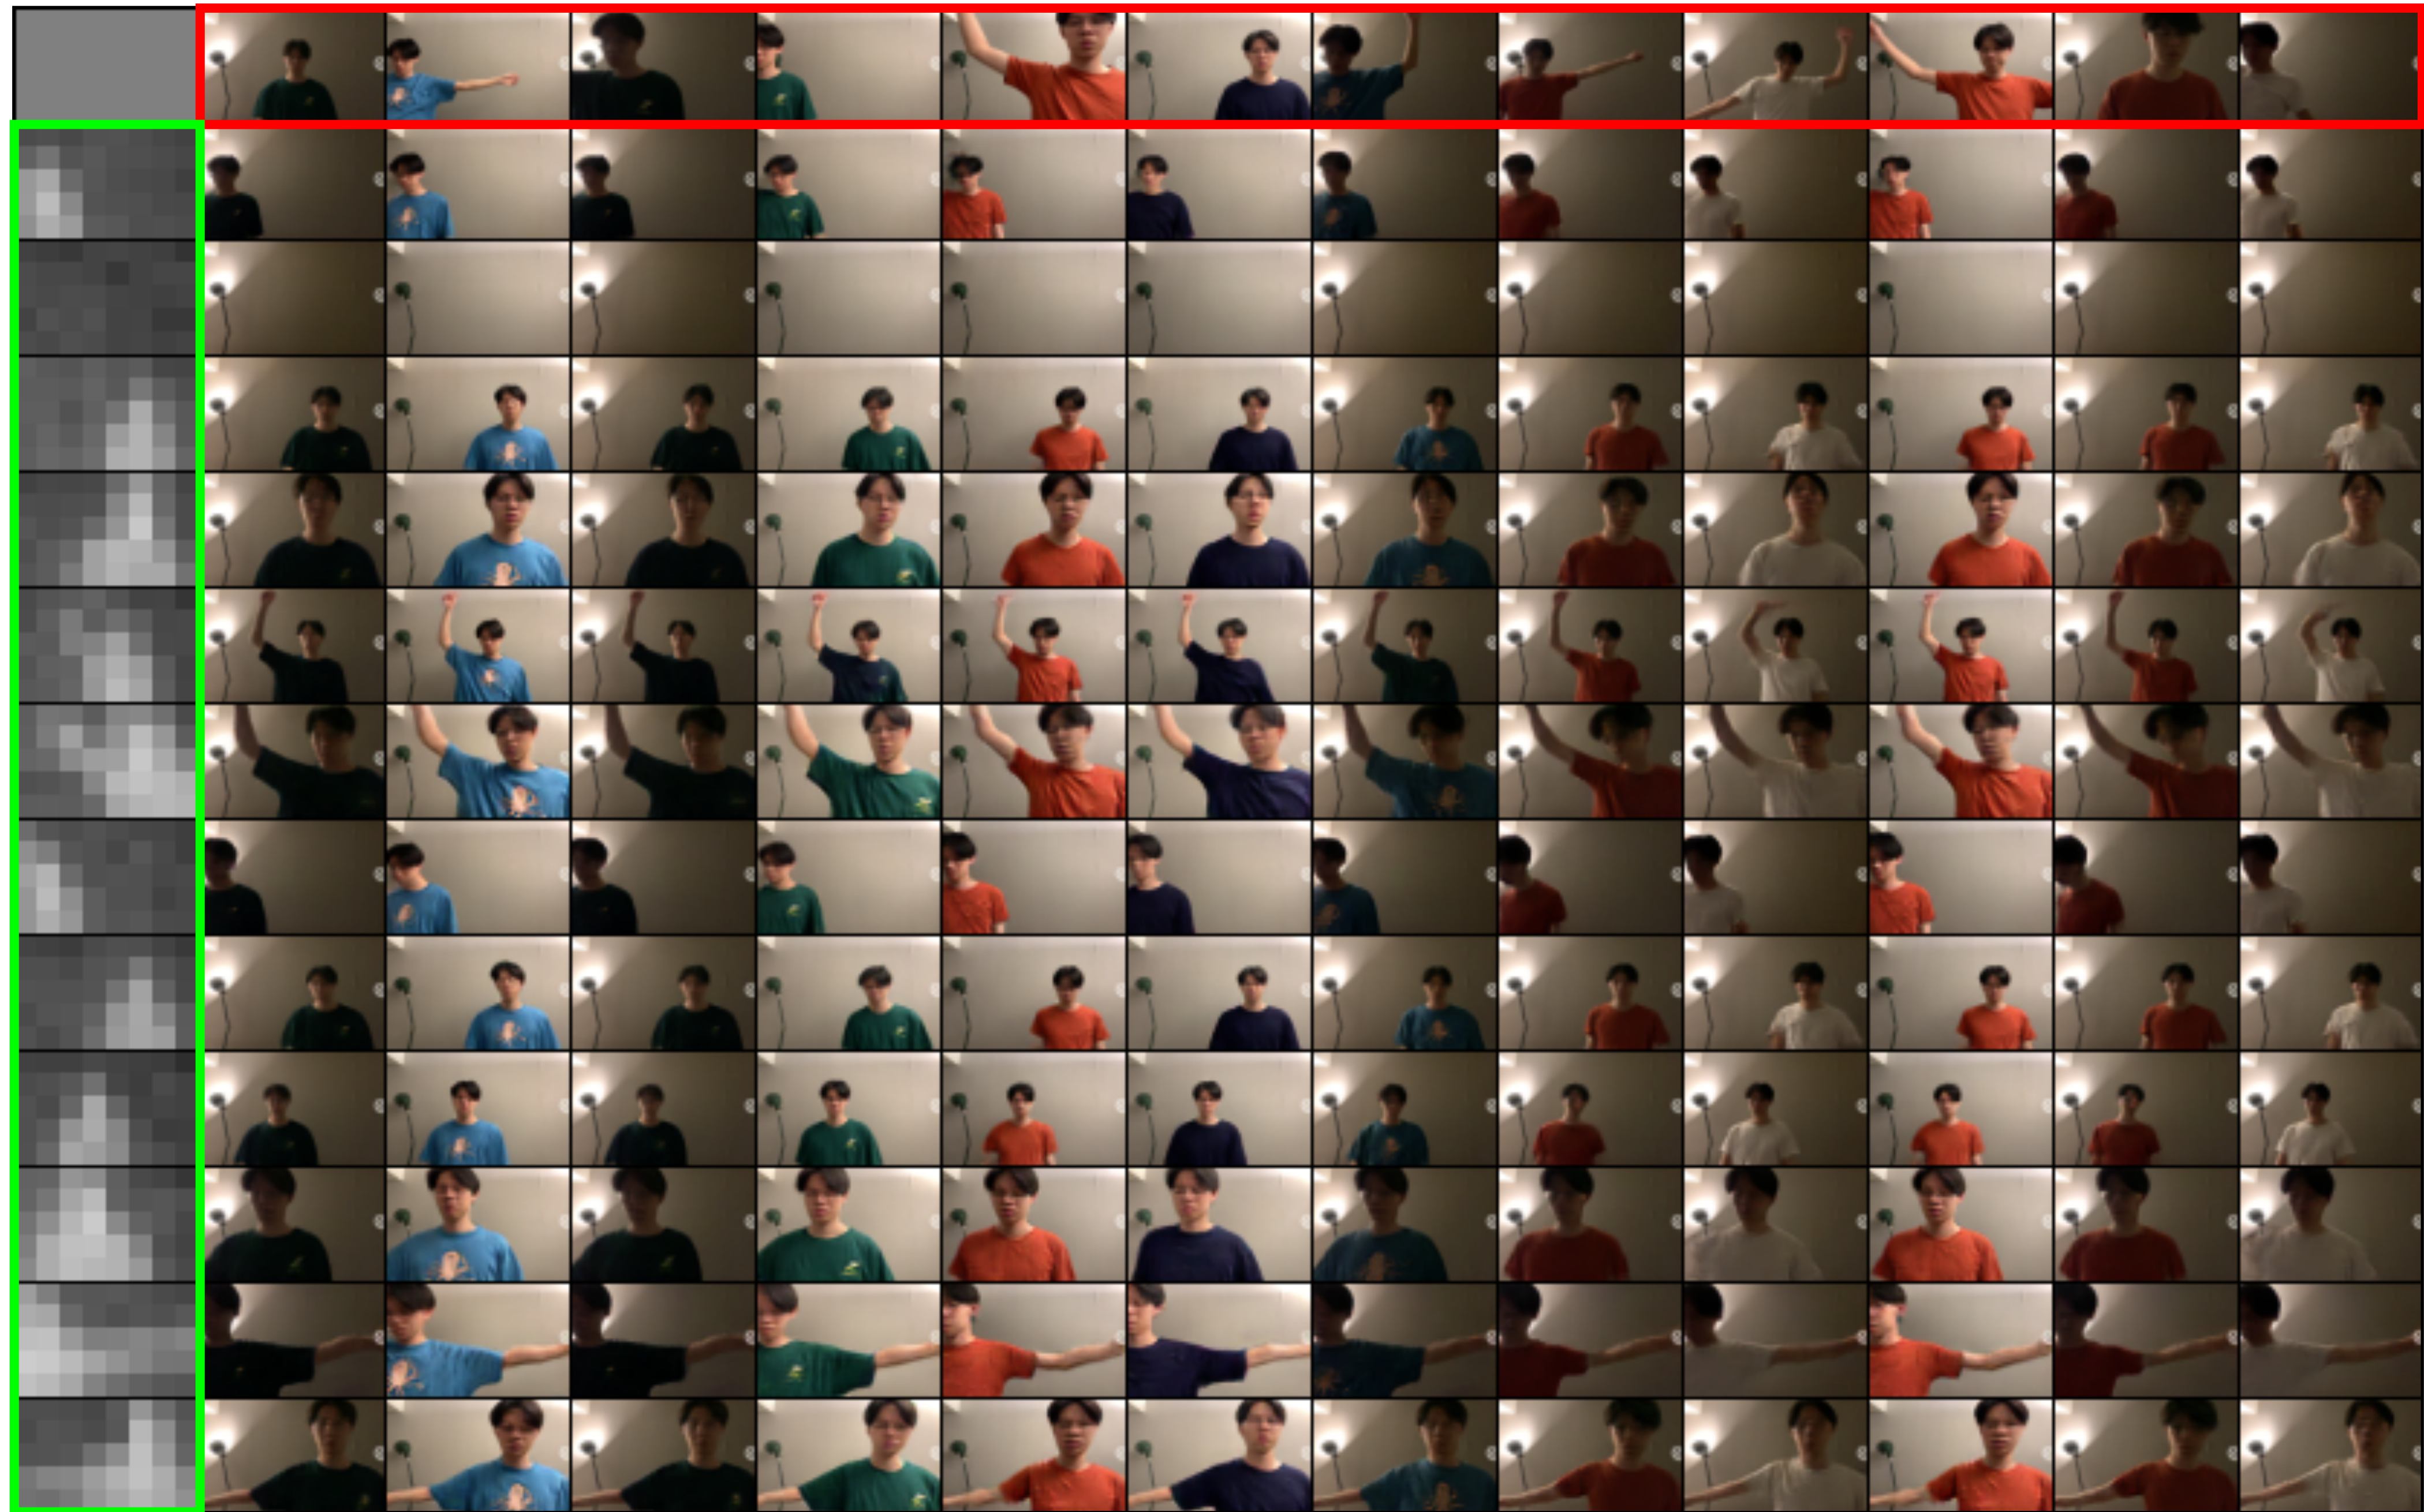



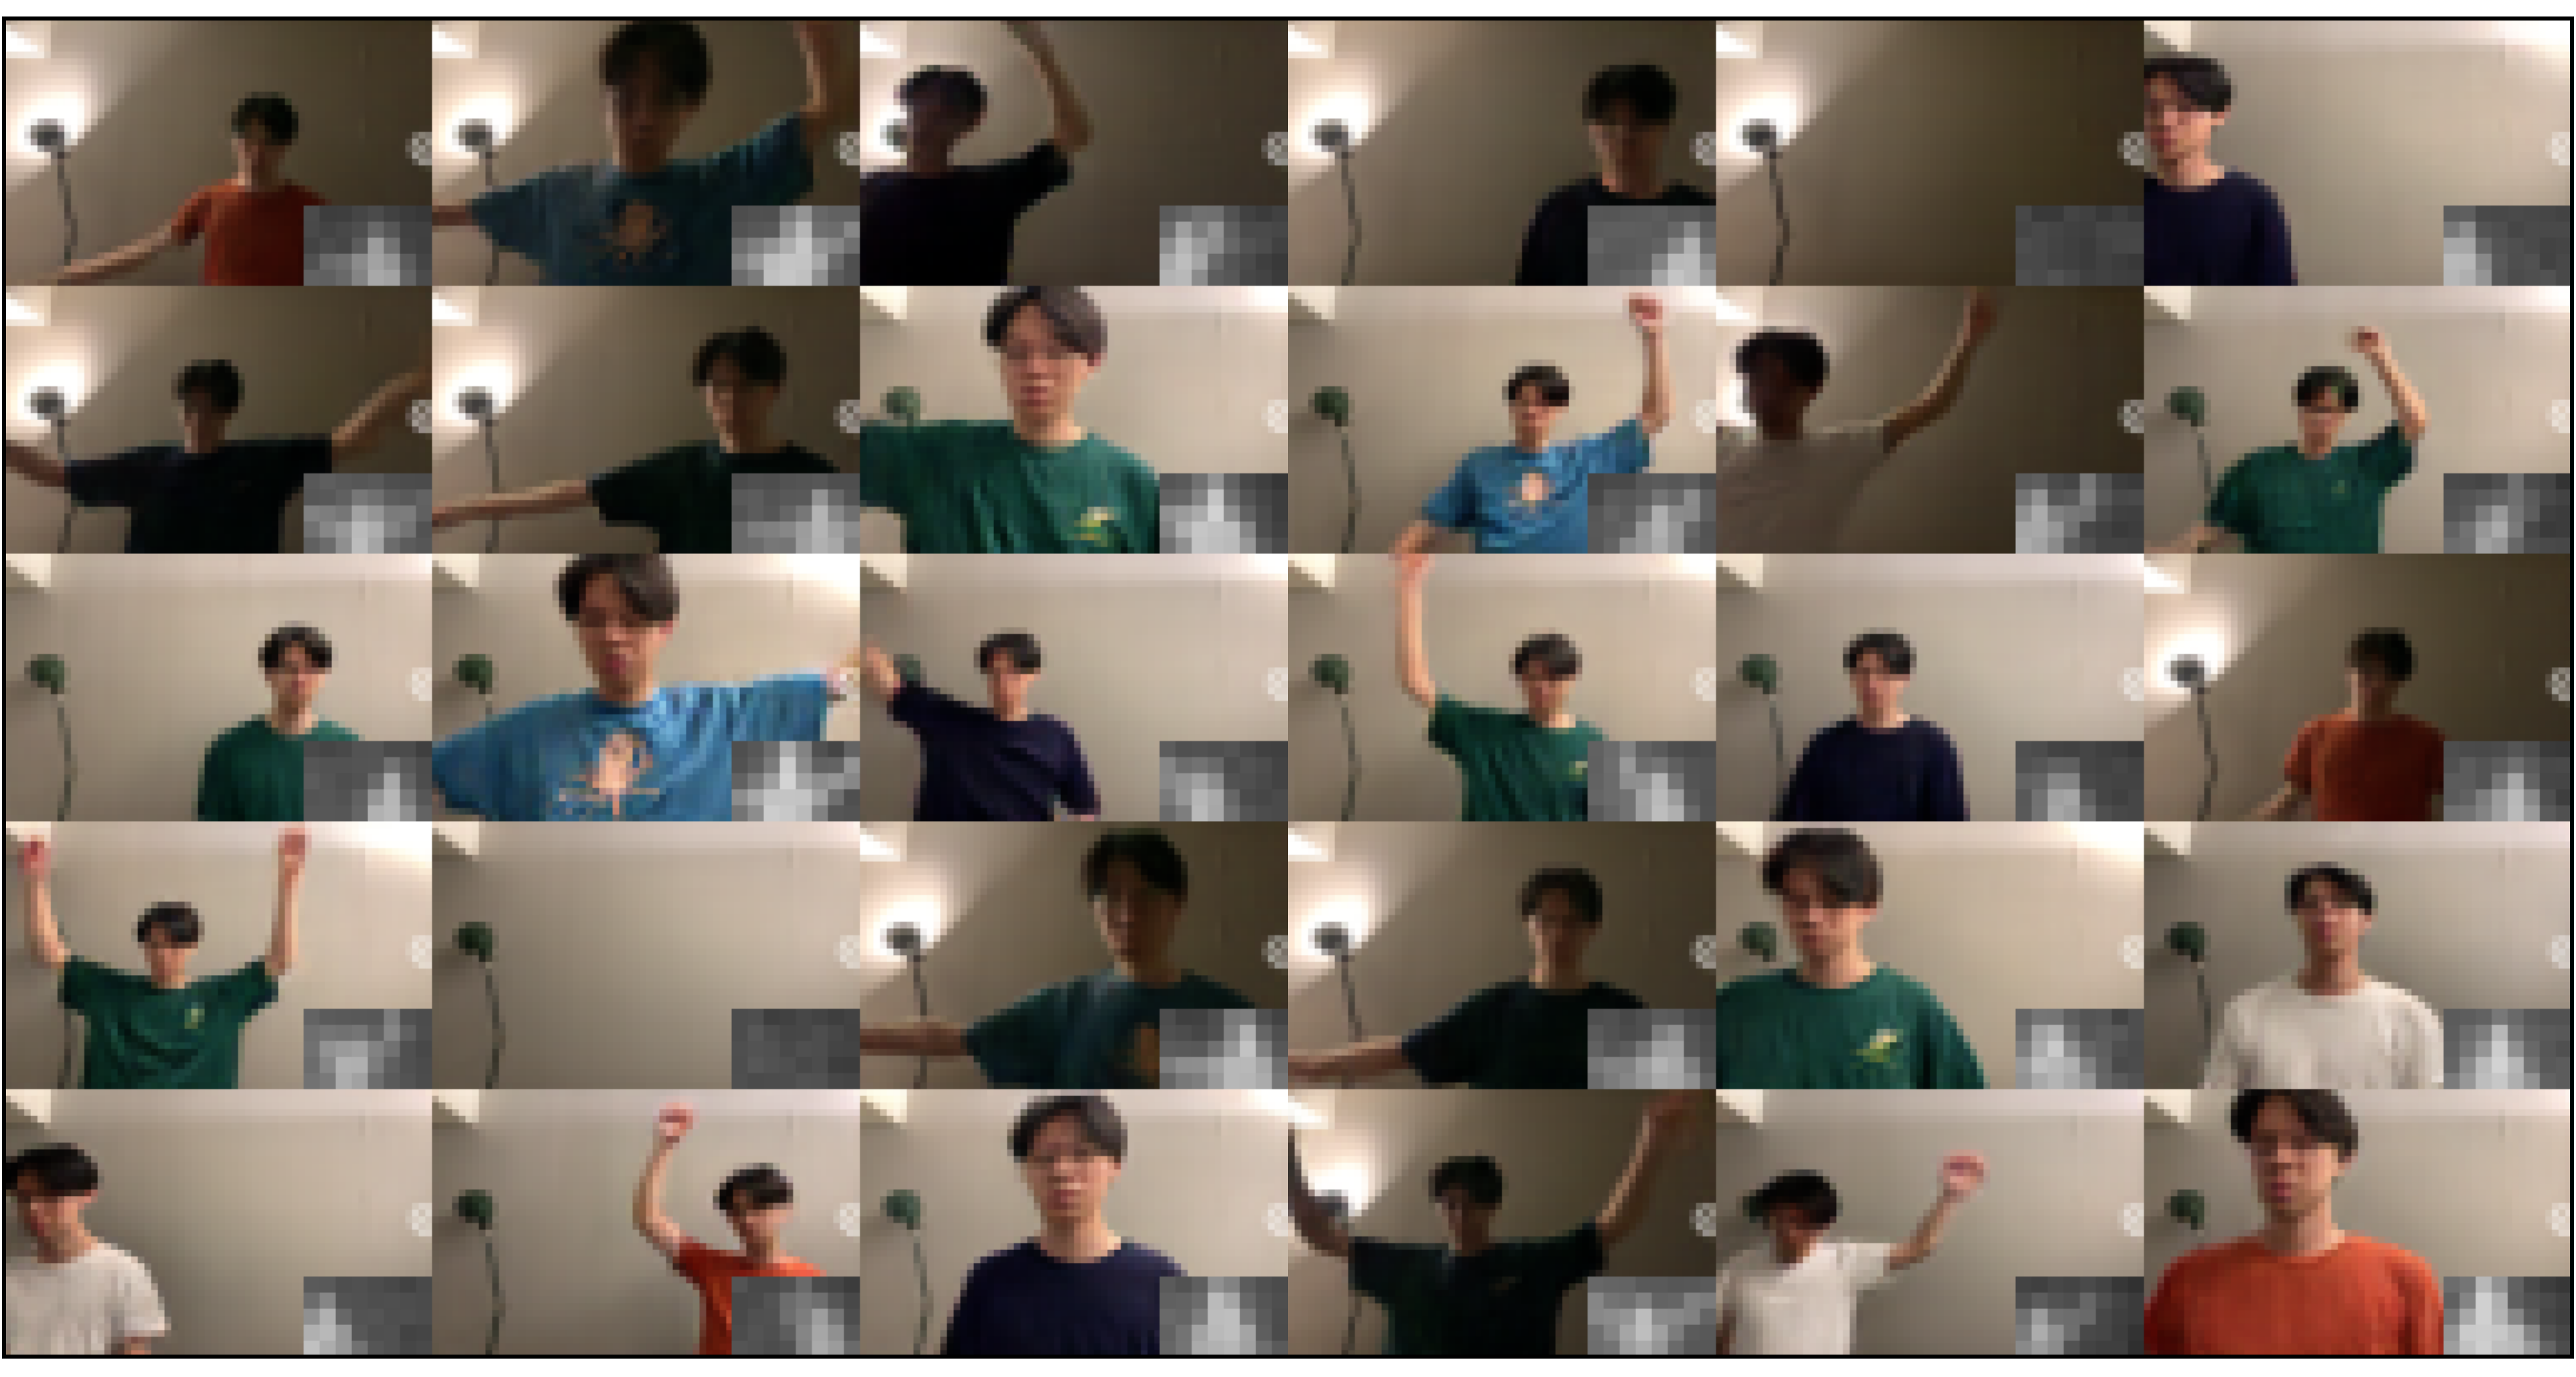

Supplement: Supplementary file 1 [file FID_SUPP.pdf]
